# Supplementary material for: Fast and Secure Decentralized Optimistic Rollups Using Setchain
Source: arXiv:2406.02316 source file (2024-06-04)
Supplement: Supplementary file 1 [file Optimistic.Client.tex]

\section{Optimistic Client Implementation}~\label{app:optimistic:client}

The client presented in this section takes advantage of
knowning processes signatures.
Instead of contacting all data committee members, it contacts the server
processes singing the batch.
% have signed it.
%
Since there are $f+1$ different signatures, it is guaranteed that at
least one of them is from a correct server, and therefore that server
will answer with the desired batch.

\begin{algorithm}[H]
\caption{\small Optmisitc client protocol for Arranger with a
    centralized Sequencer and Data Committee.}
\label{alg:client-seqDC-opt}
\small
\begin{algorithmic}[1]
\Function{\<ArrangerApi>.\textnormal{\<add>}}{$t$}
        \State \<SequencerApi>.\<Add>(t)
    \EndFunction
    \Function{\<ArrangerApi>.\textnormal{\<translate>}}{$(id,h,\textcolor{red}{sigs(id,h)})$}
                \State $\<notContacted> \leftarrow \{ p :
                sig_p(id,h) \in sigs(id,h)\}$
        \While{not received $b$ such that $\hash(b) == h$ and
        $|\<notContacted>| > 0$}
        \State take $p$ from $\<notContacted>$
        \State \<call> $p$.\<Translate>$(h)$
        \State $\<notContacted> \leftarrow \<notContacted>
        \setminus \{p\}$

        \EndWhile
        \State \<wait> for response $b$ such that $\hash(b) == h$
        \State \<return> $b$
    \EndFunction

\end{algorithmic}
\end{algorithm}
  % \vspace{-2em}
% \input{algorithms/client-seqDC-opt}
% \input{algorithms/client-setchain-opt}
\begin{algorithm}[H]
\caption{\small Optimistic client protocol for arrangers built on
    top of setchain.}
\label{alg:client-setchain-opt}
\small
\begin{algorithmic}[1]
\Function{\<ArrangerApi>.\textnormal{\<add>}}{$t$}
        \State \<call> \<Add>$(t)$ in 1 server.
    \EndFunction
    \Function{\<ArrangerApi>.\textnormal{\<translate>}}{$(id,h,sigs(id,h))$}
        \While{not received $b$ such that $\hash(b) == h$ and there
            is a server $i$ with  $sig_i(id,h) \in sigs(id,h)$ not
            contacted yet}
            \State \<call> $i.\<Translate>(id,h)$
        \EndWhile
        \State \<wait> for response $b$ such that $\hash(b) == h$
        \State \<return> $b$
    \EndFunction

\end{algorithmic}
\end{algorithm}

% Alg.~\ref{alg:client-setchain} %and Alg.~\ref{alg:client-setchain-opt}
% provide pseudo-code for a clients, similar to the one presented
% in Section~\ref{sec:seqDC}.
% %
% From the point of view of a client, the main difference with respect
% to interacting with arrangers that consist of sequencer plus data
% committee is that in decentralized arrangers all servers implement
% operation $\<add>$.
% %
% Since $f$ servers can be Byzantine, to add a new transaction $t$,
% clients invokes $\<add>(t)$ in $f+1$ servers, ensuring that at least
% one correct server is contacted.
% %
% Here we present one option, although there are other ways of
% implementing correct clients~(see
% Appendix~\ref{app:optimistic:client})

% \input{algorithms/client-setchain}
